# Supplementary material for: Optomechanical interface between telecom photons and spin quantum memory
Source: arXiv:2102.04597 ancillary file (2021-06-11)
Supplement: Supplementary file 1 [file SupplementaryInformation.pdf]

# Supplementary information for Optomechanical interface between telecom photons and spin quantum memory

Prasoon K. Shandilya,<sup>\*</sup> David P. Lake,<sup>\*</sup> Matthew J. Mitchell, Denis D. Sukachev, and Paul E. Barclay<sup>†</sup>  
*Institute for Quantum Science and Technology, University of Calgary, Calgary, Alberta T2N 1N4, Canada*  
 (Dated: June 11, 2021)

## I. EXPERIMENTAL SETUP

Measurements were performed using a home-built confocal microscope (Fig. S1a,b). A 532 nm laser (CL532-025-SO, maximum power 25 mW) and a fiber-coupled acousto-optic modulator (AOM, AAoptoelectronic MT200-BG18) generate laser pulses to prepare and readout NV spins. For imaging, we use a 100X objective lens (Nikon TU Plan ELWD, NA = 0.8) that is scanned across the sample with a 3D piezo nanopositioner (Trior 101). NV photoluminescence (PL) is separated from the 532 nm excitation with a dichroic beamsplitter, spectrally filtered (550–800 nm) and sent to a single-photon counting module (SPCM). During spin-mechanics measurements, the position of the confocal spot on the microdisk was actively stabilized based on frequently acquired photo-luminescence (PL) raster scans. -

To deliver microwave (MW) pulses, we mount the diamond sample on a custom PCB chip. A thin copper wire (diameter  $\sim 20 \mu\text{m}$ ) is placed over the sample and soldered to the PCB chip such that the wire is  $30 \mu\text{m}$  from the microdisk. MW pulses are generated by an arbitrary waveform generator (AWG, Tektronix AWG70002A) and amplified using Mini-Circuits ZHL-25W-63+. AWG marker outputs synchronize a delay generator (Stanford Research Systems DG535) used to pulse the AOM and a time-tagger (PicoQuant Timeharp 260), which builds a time-resolved histogram of photon counts from the SPCM. A DC magnetic field is produced by a permanent magnet mounted on a manual 3D translation stage. Nanopositioners (Attocube) are used to position the device and a optical fiber taper (Fig. S1a,b). The sample is positioned on an XYZ stack of slip-stick stages, while the fiber taper is mounted on an XYZ scanner stage. These stages are located within a chamber that is continuously purged with nitrogen.

To drive the mechanics in the diamond microdisk, we use a tunable diode laser (NewFocus-6700 1520-1570 nm) amplified with an erbium-doped fiber amplifier (Pritel LNHPFA-30) to  $\sim 70$  mW power. This drive laser was phase-modulated with an EOM (EOSpace PM-5S5-20-PFA-PFA-UV-UL) driven by a signal generator (Agilent N5171B) in order to injection-lock the mechanics. Another laser (NewFocus-6700 1470-1545 nm) is used to independently probe the mechanics during measurements

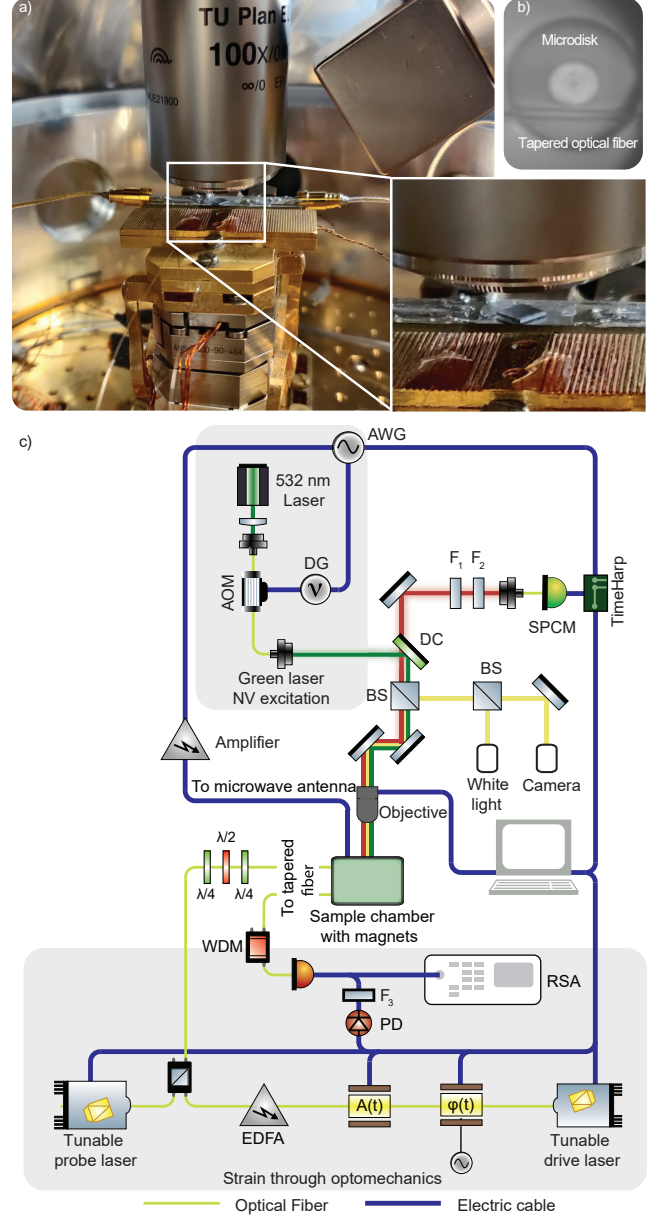

FIG. S1. Experimental setup. a) Image of the inside of the sample chamber. b) Widefield optical image of fiber taper coupled microdisk. c) Schematic of the basic setup.

where the injection locking tone is turned on. Both lasers are combined using a 90:10 fiber beam-splitter and evanescently coupled into the microdisk via the dimpled optical fiber taper.

<sup>\*</sup> These authors contributed equally

<sup>†</sup> Paul E. Barclay:Corresponding author pbarclay@ucalgary.ca

The fiber taper was created by manually pulling a standard SMF28 single mode fiber while heating it using a hydrogen torch. A dimple is created in the fiber taper so that it can be positioned in the optical near field of the microdisk without interfering with the unpatterned diamond substrate. For all of the measurements presented in the paper, the dimpled fiber taper was ‘parked’ on the shoulders of the etched circular trench that defines and surrounds the microdisk, without touching the microdisk. This ensures the stability of the tapered fiber’s position, which was not adjusted over the course of any of the measurements. The output of the fiber taper is spectrally filtered to separate the drive and probe light using a wavelength-division multiplexer (WDM: Montclair MFT-MC-51-30 AFC/AFC-1) and is monitored by a high-bandwidth photodetector (NewFocus 1554-B). The mechanical displacement of the microdisk is readout by monitoring time-dependent transmission fluctuations of drive or probe light with a real-time spectrum analyzer (Tektronix RSA5106A). To stabilize the amplitude of mechanical oscillations during the measurements, we monitor the RF power imprinted on the output light by the oscillations using a power detector (PD: Mini-Circuits ZX47-50LN-S+), and adjust the lasers’ frequency in response to slow RF power variations. We also monitor and stabilize the input power of the lasers into the fiber taper using a power meter (Newport 2936-R).

## II. DEVICE CHARACTERIZATION

### A. Device geometry

The microdisk has the diameter  $d = 5.3 \mu\text{m}$  and the thickness  $h = 0.76 \mu\text{m}$ , as measured from SEM images (Fig. S2a). It is fabricated from a single-crystal diamond chip (Element Six) with face  $\{100\}$  and edge  $\langle 100 \rangle$ . The fabrication process is described in Refs. [1, 2] where similar microdisks were fabricated and studied. Based on PL measurements performed on nominally identical samples, the NV concentration is estimated to be  $\sim 10^{13} - 10^{14} \text{ cm}^{-3}$  [3]. The microdisk is attached to the substrate via an hour-glass-shaped pedestal created during the fabrication process. This process was opti-

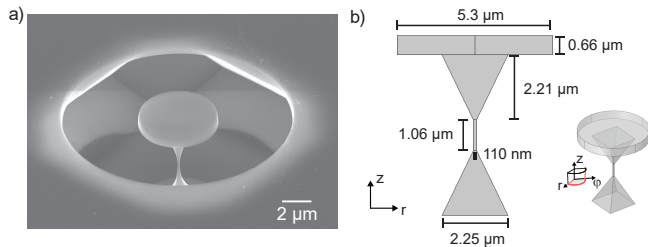

FIG. S2. a) SEM image of the microdisk. b) Model used for COMSOL simulations and the cylindrical coordinate system used throughout this paper.

TABLE S1. Microdisk parameters.

| Parameter            | Value                          | Description                                        |
|----------------------|--------------------------------|----------------------------------------------------|
| $f_m$                | 2.09 GHz <sup>a</sup>          | Mechanical frequency                               |
| $Q_m$                | 4300 <sup>a</sup>              | Mechanical quality factor                          |
| $m_{\text{eff}}$     | 19 pg <sup>b</sup>             | Effective mechanical mass                          |
| $x_{\text{zpf}}$     | 0.45 fm <sup>b</sup>           | Mechanical zero-point fluctuation amplitude        |
| $g_{\text{om}}/2\pi$ | $\sim 24.3 \text{ kHz}$ [1, 2] | Per-photon optomechanical coupling rate            |
| $G_{\text{om}}/2\pi$ | $\sim 54 \text{ GHz/nm}^b$     | Optical frequency shift per unit displacement      |
| $Q_o$                | 114000 <sup>a</sup>            | Intrinsic quality factor of the drive optical mode |
| $Q_p$                | 11000 <sup>a</sup>             | Intrinsic quality factor of probe optical mode     |
| $\lambda_o$          | 1563.71 nm <sup>a</sup>        | Center wavelength of drive mode                    |
| $\lambda_p$          | 1509.56 nm <sup>a</sup>        | Center wavelength of probe mode                    |

<sup>a</sup> Experimental value measured in this work

<sup>b</sup> Numerically simulated with COMSOL

mized to create a pedestal shape that minimizes mechanical clamping losses while providing adequate thermal management [4]. For finite-element simulations of the device’s mechanical properties, we model the pedestal as two identical pyramids and a beam. Each pyramid has a base of  $2.25 \mu\text{m} \times 2.25 \mu\text{m}$ , and the height of  $2.21 \mu\text{m}$ . Pyramids’ narrow tips connect to a beam that has the thickness of 110 nm and the length of  $1.06 \mu\text{m}$  (Fig. S2b). All relevant device parameters are summarized in Table SI.

### B. Optical properties

We use a whispering gallery mode at 1563.71 nm to optically drive the mechanics (‘drive’) and another mode at 1509.56 nm to independently probe the mechanics (‘probe’). Their transmission spectra at low laser powers with the fiber parked in the position used during

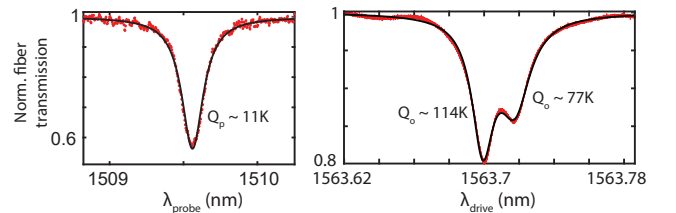

FIG. S3. Probe (left) and drive (right) whispering gallery modes of the microdisk. Intrinsic quality factors for each resonance are labeled.

the experiment are shown in Fig. S3. The relatively poor resonance contrast is due to sub-optimal fiber taper position and diameter. The drive mode has a doublet structure due to a lifted degeneracy between the microdisk's clockwise and counterclockwise propagating modes, which are coupled via back-scattering of light in the microdisk [5, 6]. By fitting the doublet with a coherent sum of two Lorentzian,

$$I(\omega) = \left| \frac{a}{1 + 2i(\omega - \omega_a)/\kappa_a} + \frac{b}{1 + 2i(\omega - \omega_b)/\kappa_b} \right|^2 \quad (1)$$

we find  $Q_o = 114000$  and  $77000$  for these standing waves. We use the higher  $Q_o$  (symmetric) mode for the optomechanical phonon excitation. The probe mode has  $Q_p = 11300$ .

### C. Optomechanical properties

To probe the optomechanical properties of the microdisk, time-dependent transmission fluctuations of the output light from the tapered fiber were monitored using a real-time spectrum analyzer. Excitation of the microdisk mechanical resonance modulates the wavelength of the microdisk's optical modes via a dispersive optomechanical coupling quantified by  $g_{om}$  given in Table SI. When the laser wavelength is tuned near the optical cavity resonance, the mechanical motion is optomechanically transduced to the optical signal that can be observed by measuring the photodetected electronic power spectrum ( $S_p$ ). Figure S4a shows a typical spectrum of mechanical motion when the laser wavelength is tuned to the point where cavity slope is maximum—the point of maximum transduction of the modes in Fig. S3. The observed resonance near frequency  $\sim 2.09$  GHz (quality factor  $\sim 4,300$ ) corresponds to the fundamental radial breathing mode (RBM) of the microdisk.

The transduced mechanical signal for varying optical power launched ( $P$ ) into the microdisk shows a transi-

tion from thermal motion to self-oscillation (Fig. S4b). During this measurement, the drive laser's wavelength was tuned to the value of maximum transduction at each power setting to account for thermo-optic dispersion of the optical mode wavelength. As  $P$  increases the mechanical resonance narrows and increases in amplitude, and exhibits the onset of self-oscillations, also referred to as phonon lasing. Using  $P$  and the cavity transmission normalized to the input power ( $\bar{T}$ ), we can calculate the power dropped into the microdisk drive mode given by  $P_d = (1 - \bar{T})P$ .

At low power, the mechanical motion of the microdisk (Fig. S4a) is dominantly from the thermal bath, and its r.m.s. mechanical displacement is predicted from the equipartition theorem to be [7]:

$$x_{th} = \sqrt{\frac{k_B T}{m_{eff} \omega_m^2}} \quad (2)$$

where  $k_B$  is the Boltzmann constant,  $T = 295$  K is the bath temperature,  $\omega_m/2\pi \sim 2.1$  GHz is the measured mechanical frequency of the RBM, and the effective mass  $m_{eff} = 19$  pg is predicted from finite element simulations. This results in  $x_{th} \sim 25$  fm and corresponding zero point fluctuation amplitude  $x_{zpf} \sim 0.45$  fm. The maximum displacement amplitude ( $x_{so}$ ) of the RBM in the self-oscillation regime is given by [1]:

$$x_{so} = x_{th} \sqrt{\frac{A_{so} P_{th}^2}{A_{th} P_{so}^2}} \quad (3)$$

where  $A_{so}$  and  $A_{th}$  are the areas under the curves in the self-oscillating ( $P_d = P_{so}$ ) and thermal ( $P_d = P_{th}$ ) states, respectively. For the self-oscillation measurements presented here, this results in  $x_{so} \sim 9$  pm. Using the value obtained for  $x_{so}$ , we can estimate the number of phonons in the self-oscillating regime ( $N_{max}$ ) using the relation  $x_{so} = \sqrt{N_{max}} \times x_{zpf}$  which gives  $N_{max} \approx 4 \times 10^8$  phonons.

For measurements involving injection locking (Fig. 2d,e and Fig. 4 in the main text), we use the probe laser to independently measure the mechanical oscillations. This is necessary to unambiguously separate the contributions to the measured electronic spectrum due to mechanical motion from those created by the phase modulation. The energy of mechanical self-oscillations, measured via the optically-transduced power spectral density, is observed to decrease as  $|\delta_{m,i}|$  ( $\delta_{m,i} = \omega_m - \omega_{inj}$ ) increases (see Fig. 2e in the main text). This dependence has a Lorentzian profile with a FWHM = 380 kHz. Since the mechanical energy scales quadratically with the dynamical stress produced by the RBM, the latter will have a square root of Lorentzian dependence on  $\delta_{m,i}/2\pi$  with a FWHM of  $\sqrt{3} \times 380$  kHz.

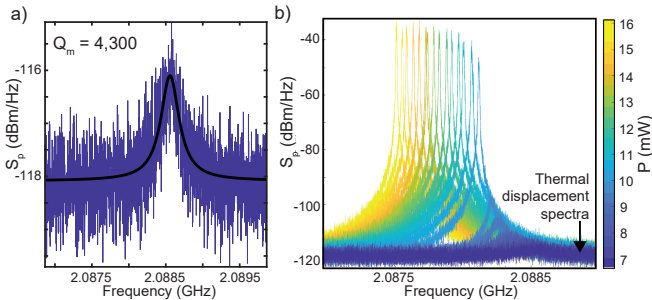

FIG. S4. a) Power spectral density (PSD) of thermal displacement associated with the RBM with a Lorentzian fit (black). b) PSD of the mechanical motion for varying laser drive power input to the fiber taper showing the onset of self-oscillations. Each spectrum has been horizontally shifted by  $\sim 0.04$  MHz for better visibility.

### III. NV ENSEMBLE CHARACTERIZATION AND MICROWAVE CONTROL

#### A. NV spin initialization and readout

The NV spin is initialized into the  $m_s = 0$  spin state via optical pumping using a  $5 \mu\text{s}$ -long  $532 \text{ nm}$  laser pulse. A similar laser pulse is used to read out the NV spin state via spin-dependent photo-luminescence (PL) [8].

As a readout signal  $S$  we use the number of photons detected during the first  $250 \text{ ns}$  of time-resolved PL, normalized to the number of photons at the end of  $5 \mu\text{s}$ -long readout pulse. This measurement is then averaged over many repetitions. This scheme allows determination of the population in  $|0\rangle$ , but cannot differentiate between population in the  $|\pm 1\rangle$  states due to their similar PL signals. Thus, we readout the populations  $p_{\pm 1}$  of  $|\pm 1\rangle$  states differently: we first move spins from  $|+1\rangle$  or  $|-1\rangle$  to  $|0\rangle$  with a resonant MW  $\pi$ -pulse, and then use the readout scheme described above.

#### B. Microwave control

To select a single orientation of spins to resonantly couple to the mechanical resonator, we align the external magnetic field along the NV axis by maximizing the CW fluorescence counts under green excitation [8]. The resonant frequency of the  $|0\rangle \rightarrow |\pm 1\rangle$  transitions and the splitting between the  $|\pm 1\rangle$  levels is precisely determined using optically-detected magnetic resonance (ODMR) measurements shown in Fig. S5. The observed triplet structure for each electronic state in the ODMR spectrum is due to hyperfine coupling of NV electronic spins to  $^{14}\text{N}$  nuclear spin. The asymmetry in the depth of the ODMR triplets comes from a partial nuclear spin polarization due to a level anticrossing in the NV excited state that occurs at a magnetic field of  $500 \text{ G}$  [9, 10] that is relatively close the  $350 \text{ G}$  field used to split the  $|\pm 1\rangle$  states by the  $2.1 \text{ GHz}$  mechanical frequency.

The state of the electronic spin qubit is controlled by applying microwave (MW) pulses resonant with spin transitions. Figures S6(a,b) show Rabi oscillations of the

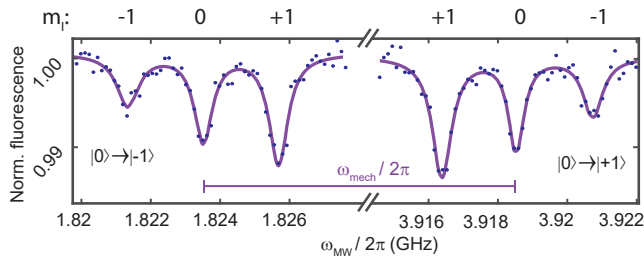

FIG. S5. Pulsed optically-detected magnetic resonances. Numbers on the top denote nuclear spin projection which is preserved under MW drive.

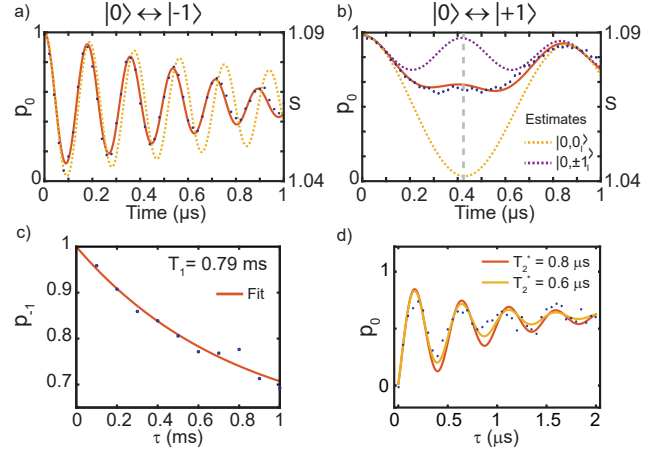

FIG. S6. Characterization of the NV ensemble. a,b) Rabi oscillations on  $|0\rangle \leftrightarrow |\pm 1\rangle$  transitions. Solid red lines are fits including all three hyperfine sublevels, yellow and purple dashed lines are the populations of  $|0, 0_I\rangle$  and  $|0, \pm 1_I\rangle$  level inferred from the fits.  $S$  refers to the readout signal of the measured Rabi oscillation. c)  $T_1$  measurements of NV ensemble. d) Ramsey experiment alongside theoretical model for two values of  $T_2^* = 0.6$  and  $0.8 \mu\text{s}$ .

electronic spin between the  $|0\rangle \leftrightarrow |-1\rangle$  and  $|0\rangle \leftrightarrow |+1\rangle$  states, respectively. We use these oscillations to calibrate the readout signal, and plot them both in terms of spin state populations (left axis) and measured signal (right axis). To convert signal to population, we first assume that the green pulse initializes all spins in  $|0\rangle$  (below we will lift this restriction), which means that the signal value of  $S_0 \approx 1.09$  corresponds to NVs being in the state  $|0\rangle$ . If the Rabi frequency ( $5 \text{ MHz}$  here) is higher than the dephasing rate ( $1 \text{ MHz}$ ) and the detuning from the resonance ( $< 100 \text{ kHz}$ ) then spin population will transition between the states  $|0\rangle$  and  $|-1\rangle$  with a 100% contrast. This allows us to determine that  $S_{-1} \approx 1.04$  denotes NVs being in the state  $|-1\rangle$ . Using this, we find the probability of NVs being in the  $|0\rangle$  state for an arbitrary  $S$ :

$$p_0 = (S - S_{-1}) / (S_0 - S_{-1}), \quad (4)$$

and  $p_{+1} + p_{-1} = 1 - p_0$ .

It is known that the fidelity of the NV spin initialization with green light is not 100% but is closer to 80%. Since this uncertainty equally affects the MW Rabi oscillation and the optomechanical driving signal contrasts, non-perfect spin initialization does not interfere with our ability to determine the strength of the optomechanical driving. Also, after initialization, some NVs can be in the unsuitable charge state (neutrally charged  $\text{NV}^0$ ), which is not affected by the mechanics but fluoresces under green illumination. We assume that the charge state does not change during the  $7 \mu\text{s}$ -long mechanical driving time. This is supported by our observation that the PL signal does not change during this time when no driving fields (MW, mechanics) are applied. This constant  $\text{NV}^0$

signal adds to  $S$  and is canceled when we find  $p_0$  (see Eq. S4).

Frequency dispersion in the MW antenna response causes different Rabi frequencies for the two transitions used in our scheme. At the maximum MW power, the  $|0\rangle \rightarrow |-1\rangle$  Rabi frequency is 9 MHz, which is fast enough to equally drive all three hyperfine sublevels (Fig. S6a). However, the  $|0\rangle \rightarrow |+1\rangle$  Rabi frequency is only 2 MHz, which is comparable to the splitting of 2.1 MHz between triplet components and thus drives them unequally (Fig. S6b). In this regime, a  $\pi$ -pulse for the  $|0, 0_I\rangle \rightarrow |+1, 0_I\rangle$  transition will result in a power dependent rotation between the off-resonance  $\pm 1_I$  hyperfine sublevels, leaving them in a superposition of  $|0, \pm 1_I\rangle$  and  $|+1, \pm 1_I\rangle$ . To avoid this and simplify the analysis, we implemented a ‘magic’  $\pi$ -pulse. We adjusted the MW power so that the generalized Rabi frequency, which includes the frequency detuning, for the transition  $|0, \pm 1_I\rangle \rightarrow |+1, \pm 1_I\rangle$  is twice as fast as for the transition of interest  $|0, 0_I\rangle \rightarrow |+1, 0_I\rangle$ . Thus, a  $\pi$ -pulse for  $|0, 0_I\rangle \rightarrow |+1, 0_I\rangle$  will correspond to a  $2\pi$ -pulse for  $|0, 1_I\rangle \rightarrow |+1, 1_I\rangle$  (Fig. S6b), effectively leaving the  $|\pm 1_I\rangle$  sublevels unaffected. The effect of the ‘magic’  $\pi$ -pulse is reflected in the reduced contrast in Fig. S6b, which is  $1/3$  of the contrast in Fig. S6a. To more precisely evaluate the efficacy of this approach, we fit the measured  $p_0$  data to a model taking into account all three hyperfine sublevels of each electronic state with their relative weights obtained from the ODMR spectra (see Fig. S5). We find excellent agreement, and can extract the populations in the  $|0, \pm 1_I\rangle$  and  $|0, 0_I\rangle$  states, confirming that when the maximum population has been transferred out of  $|0, 0_I\rangle$ , the  $|\pm 1, 0_I\rangle$  populations are nearly unchanged.

Note that achieving higher Rabi frequencies, which would eliminate the need to use a magic  $\pi$ -pulse, requires moving the wire closer to the microdisk, or increasing the input microwave power. Both adjustments come with the risk of damaging the device or wire and therefore were not pursued.

We measured a relaxation time  $T_1 \approx 600 \mu\text{s}$  (Fig. S6c) for the  $|\pm 1\rangle$  states of the NV ensemble used in this work. To find the ensemble spin coherence time we did Ramsey measurements between the  $|0\rangle$  and  $|-1\rangle$  levels (Fig. S6d). Fitting the data with the model introduced above, we determine that any coherence time in the interval  $T_2^* = 0.6 - 0.8 \mu\text{s}$  fits the data equally well. These numbers are typical for optical grade diamond samples [11]. As shown in Fig. 4d from the main text, this precision is enough to infer from the model the mechanical Rabi frequency  $\Omega_m$ . The measured  $T_2^*$  time corresponds to a FWHM of the ODMR resonances of  $1/(\pi T_2^*) = 400 - 540 \text{ kHz}$  which is close to the measured width of 610 kHz (Fig. S5). The difference can be explained by the residual power broadening.

We have also checked numerically that performance of the  $\pi$ -pulses is not degraded by the continuous strain driving field, as the MW Rabi frequencies are large compared with the estimated mechanical Rabi frequency of

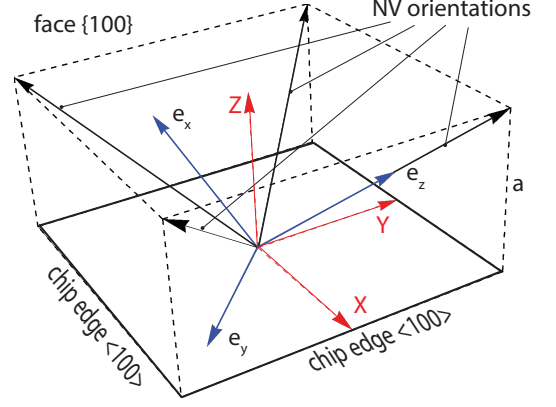

FIG. S7. Relative orientation of the diamond chip (bottom rectangular), showing the 4 possible NV orientations (black arrows) in the laboratory frame (red) and the NV frame (blue). The magnetic field is aligned along  $e_z$ .

$< 200 \text{ kHz}$  (see Fig. 4 in the main text).

## IV. MECHANICAL SPIN CONTROL

### A. NV-stress Hamiltonian

To analyze the spin-stress Hamiltonian, we follow Ref. [12]. We choose a Cartesian reference frame centred at the vacancy, with the nitrogen impurity at the point  $(a/4, a/4, a/4)$ , with  $a$  being the lattice constant. It is natural to express the stress in the frame associated with the NV centers (see Fig. S7). We use three orthogonal basis vectors  $e_z = (1, 1, 1)/\sqrt{3}$ ,  $e_y = (1, -1, 0)/\sqrt{2}$ , and  $e_x = e_y \times e_z$ . Of course, due to the  $C_{3v}$  symmetry of the NV centers, we can rotate this frame by  $\pm 2\pi/3$  around  $e_z$  and get the same end results. In the chosen basis, the NV-stress Hamiltonian reads:

$$H_\sigma = H_{\sigma 0} + H_{\sigma 1} + H_{\sigma 2}, \quad (5)$$

$$H_{\sigma 0}/\hbar = [g_{41}(\sigma_{xx} + \sigma_{yy}) + g_{43}\sigma_{zz}] S_z^2, \quad (6)$$

$$H_{\sigma 1}/\hbar = \frac{1}{2} \left[ g_{26}\sigma_{xz} - \frac{1}{2}g_{25}(\sigma_{xx} - \sigma_{yy}) \right] \{S_x, S_z\} + \frac{1}{2}(g_{26}\sigma_{yz} + g_{25}\sigma_{xy})\{S_y, S_z\}, \quad (7)$$

$$H_{\sigma 2}/\hbar = \frac{1}{2} \left[ g_{16}\sigma_{xz} - \frac{1}{2}g_{15}(\sigma_{xx} - \sigma_{yy}) \right] (S_y^2 - S_x^2) + \frac{1}{2}(g_{16}\sigma_{yz} + g_{15}\sigma_{xy})\{S_x, S_y\}, \quad (8)$$

where:

$$\{A, B\} = AB + BA. \quad (9)$$

The stress-coupling parameters  $g_{ij}$  (along with strain-coupling coefficients  $h_{ij}$ ) are summarized in Table S2. The  $H_{\sigma 0}$  Hamiltonian only results in a symmetrical shift

TABLE S2. Spin-strain ( $h$ ) and spin-stress ( $g$ ) coupling-strength parameters for the NV ground state calculated from density functional theory in Ref. [12].

| Parameter | Value (MHz/strain) | Parameter | Value (MHz/GPa)  |
|-----------|--------------------|-----------|------------------|
| $h_{43}$  | $2300 \pm 200$     | $g_{43}$  | $2.4 \pm 0.2$    |
| $h_{41}$  | $-6420 \pm 90$     | $g_{41}$  | $-5.17 \pm 0.07$ |
| $h_{25}$  | $-2600 \pm 80$     | $g_{25}$  | $-2.17 \pm 0.07$ |
| $h_{26}$  | $-2830 \pm 70$     | $g_{26}$  | $-2.58 \pm 0.06$ |
| $h_{15}$  | $5700 \pm 200$     | $g_{15}$  | $3.6 \pm 0.1$    |
| $h_{16}$  | $19660 \pm 90$     | $g_{16}$  | $18.98 \pm 0.09$ |

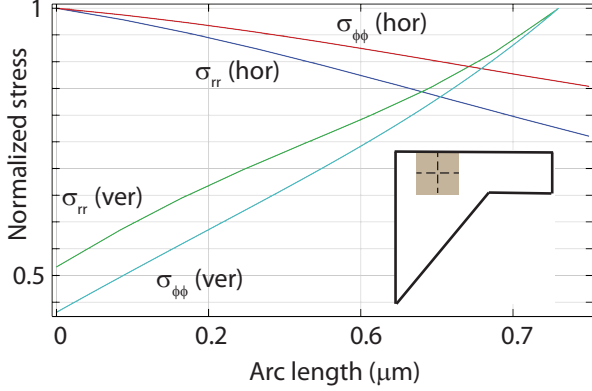

FIG. S8. Vertical and horizontal profiles (dashed lines in the inset) of  $\sigma_{r,r}$  and  $\sigma_{\phi,\phi}$  stress components over the confocal volume (gray region in the inset).

of NV  $|\pm 1\rangle$  levels and is not relevant to our work.  $H_{\sigma 1}$  couples level  $|0\rangle$  to levels  $|\pm 1\rangle$  via stress, while  $H_{\sigma 2}$  causes the transition  $|+1\rangle \rightarrow |-1\rangle$ . Since the corresponding coupling parameters  $g_{15}$  and  $g_{16}$  are much greater than  $g_{25}$  and  $g_{26}$  we focus on the  $|+1\rangle \rightarrow |-1\rangle$  transition in this experiment.

### B. NV-phonon coupling rates

At our collection spot ( $0.7 \mu\text{m}$  away from the microdisk center), the simulated stress tensor per single phonon in the microdisk coordinates  $(\hat{r}, \hat{\phi}, \hat{z})$  is:

$$\sigma_0 \approx \begin{pmatrix} 689 & 0 & -1 \\ 0 & 832 & 0 \\ -1 & 0 & 1 \end{pmatrix} \text{ Pa.} \quad (10)$$

Stress in the microdisk is extremely non-homogeneous (see Fig. 2a in the main text). Thus, after averaging over a  $\sim 1 \mu\text{m}^3$  confocal volume (Fig. S8) the stress is reduced by  $\sim 30\%$ :

$$\sigma_{\text{avg}} \approx \begin{pmatrix} 523 & 0 & -93 \\ 0 & 562 & 0 \\ -93 & 0 & -84 \end{pmatrix} \text{ Pa.} \quad (11)$$

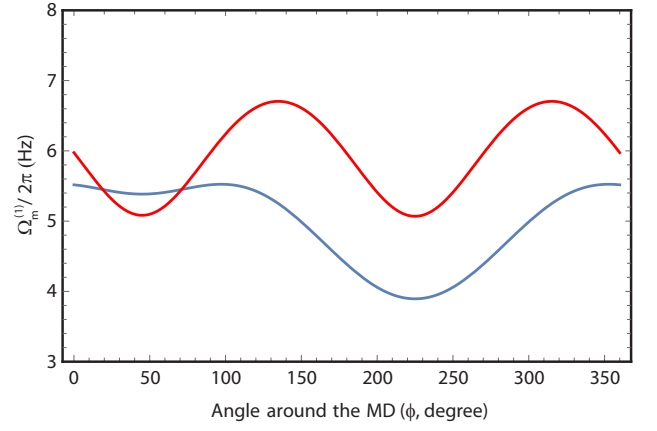

FIG. S9. Single-phonon Rabi freq  $\Omega_m^{(1)}/2\pi$  as a function of the angle  $\phi$  at the 'point of interest' on the microdisk (red) that is  $0.7 \mu\text{m}$  off the center; blue curve takes into account averaging over the 'confocal' volume.

To find NV-stress coupling rates, we rewrite the stress tensor in the NV coordinate frame  $(e_x, e_y, e_z)$  introduced above and get:

$$\begin{pmatrix} 234 & -18 & -328 \\ -18 & 825 & 26 \\ -328 & 26 & 464 \end{pmatrix} \text{ Pa.} \quad (12)$$

Next, we chose a position on the disk along the  $\hat{\phi}$  coordinate. Fig. S9 plots the angular dependence of the single-phonon Rabi frequency for the stress tensors  $\sigma_0$  (red) and  $\sigma_{\text{avg}}$  (blue). The asymmetry in Fig. S9 originates from the change of the orientation of the NV symmetry axis (coordinate frame  $(e_x, e_y, e_z)$ ) with respect to the local coordinate frame of the microdisk  $((\hat{r}, \hat{\phi}, \hat{z}))$  when the angle  $\phi$  is varied. We work at  $\phi \sim 45^\circ$  where the single-phonon Rabi frequency  $\Omega_m^{(1)}/2\pi = 5.5 \text{ Hz}$ . Rabi frequency scales with the number of phonons in the mode  $N$  as:

$$\Omega_m = \Omega_m^{(1)} \times \sqrt{N}. \quad (13)$$

In Sec. II C we estimate  $N_{\text{max}} \sim 4 \times 10^8$  phonons in the self-oscillation regime, which corresponds to  $\Omega_m^{\text{max}}/2\pi \approx 110 \text{ kHz}$ .

### C. Quantum master equation

In order to infer stress-coupling rates from our experimental data, we numerically simulated the dynamics of an NV ensemble under a mechanical drive. We begin with the Hamiltonian,

$$H = H_0 + H_B + H_{\sigma 0} + H_{\sigma 1} + H_{\sigma 2}, \quad (14)$$

where:

$$H_0/h = D_0 S_z^2, \quad (15)$$

is the NV Hamiltonian with zero-field splitting  $D_0 = 2.87$  GHz. The external magnetic field is taken into account with:

$$H_B/h = g_e \vec{S} \cdot \vec{B}, \quad (16)$$

where  $g_e = 2.8$  MHz/G is NV spin gyromagnetic ratio and  $\vec{S} = (S_x, S_y, S_z)$ . The quantum master equation for the density matrix  $\rho$  reads:

$$i\hbar\rho'(t) = [H, \rho(t)] + \sum_{i,j} L_{i,j}[\rho], \quad (17)$$

where  $L_{i,j}[\cdot]$  are Lindblad superoperators describing longitudinal ( $T_1$ ) and transverse ( $T_2^*$ ) decays of the density matrix, and have the form:

$$L_{i,j}[\rho] = \hbar\Gamma_{i,j} \left( O_{i,j}\rho O_{i,j}^\dagger - \frac{1}{2} \{O_{i,j}^\dagger O_{i,j}, \rho\} \right), \quad (18)$$

where  $O_{i,j} = |i\rangle\langle j|$  are quantum jump operators from state  $|j\rangle$  to state  $|i\rangle$ . Although it is hard to deduce longitudinal relaxation coefficients  $\{\Gamma_{i,i}\}$  for each level from the data in Fig. S6, it is clear that all of them are longer than  $100 \mu\text{s}$  and do not affect the dynamics on the shorter times ( $< 7 \mu\text{s}$ ) that are relevant for this work. Thus we assume they are equal:

$$\Gamma_{i,j} = 1/(3T_1), i \neq j \quad (19)$$

where  $T_1$  is the population relaxation coefficient measured in Fig. S6c. We also assume that magnetic noise dominates the NV spin dephasing and let:

$$\Gamma_{-1,-1} = \Gamma_{+1,+1} = 2/T_2^*, \Gamma_{0,0} = 0, \quad (20)$$

where  $T_2^*$  is Ramsey coherence time on the  $|0\rangle \rightarrow |\pm 1\rangle$  transitions. This takes into account that the transition of interest  $|+1\rangle \rightarrow |-1\rangle$  dephases twice as fast as transitions  $|0\rangle \rightarrow |\pm 1\rangle$ .

Since stress-coupling coefficients  $g_{4,1}$  and  $g_{4,3}$  are much smaller than  $g_{1,6}$ ,  $H_{\sigma 0}$  does not affect the dynamics and was omitted from the simulations. The  $H_{\sigma 1}$  term couples level  $|0\rangle$  to levels  $|\pm 1\rangle$  and will be far off-resonant:  $f_{0 \rightarrow +1(-1)} = 1.8(3.9)$  GHz which is far-detuned from  $f_m = 2.1$  GHz and can be omitted as well.

In the rotating wave approximation:

$$H = H_{\sigma 2} = \hbar \begin{pmatrix} 0 & 0 & \Omega_m/2 \\ 0 & 0 & 0 \\ \Omega_m^\dagger/2 & 0 & \delta_{s,i} \end{pmatrix} \quad (21)$$

where

$$\Omega_m = \left( \frac{1}{2} g_{15}(\sigma_{xx} - \sigma_{yy}) - \sigma_{zx} g_{16} \right) - i(\sigma_{xy} g_{15} + \sigma_{yz} g_{16}) \quad (22)$$

is the mechanical Rabi frequency and  $\delta_{s,i}$  is the detuning between the NV spin transition and the locked mechanical frequency (both are in angular frequency units).

## D. Time-resolved dynamics

Even though we carried out measurements in the spectral domain (Fig. 4), it is insightful to conduct numerical simulations in the time domain. Figure S10 shows the population  $p_{-1}$  transferred to state  $|-1\rangle$  after time  $t$  of mechanical driving with  $\Omega_m/2\pi = 150$  and  $1500$  kHz when the NV is initially polarized to state  $|+1\rangle$ .

For  $\Omega_m/2\pi \approx 150$  kHz expected for our system, the dynamics of  $p_{-1}$  do not show any oscillations since  $\Omega_m < 1/T_2^*$ . Instead, it first monotonically approaches  $p_{-1} \approx 0.5$  on a  $\sim 10 \mu\text{s}$  time-scale and then decreases to a steady-state value of  $1/3$  due to  $T_1$  relaxation (Fig. S10 inset). For the optomechanical spin driving measurements in Fig. 4 we let the mechanics interact with NVs for  $t = 7 \mu\text{s}$  (dashed vertical line in Fig. S10). This  $t$  is a compromise between having a reasonable value of  $p_{-1}$  and keeping the acquisition time short enough to avoid drifts in experimental parameters. Figure S10 also shows that for detuning  $\delta_{s,i} > \Omega_m$ , the change in  $p_{-1}$  is significantly reduced, as expected for a non-resonant drive.

We would like to note that due to spatial variations of the stress over the confocal volume (Fig. S8),  $\Omega_m$  of individual NV centers can vary by  $\pm 15\%$ . Since this variation is too small to affect the time dynamics of the signal in Fig. S10, we do not take into account these microscopic details of the NV-phonon coupling but instead use an effective Rabi frequency averaged over the confocal volume.

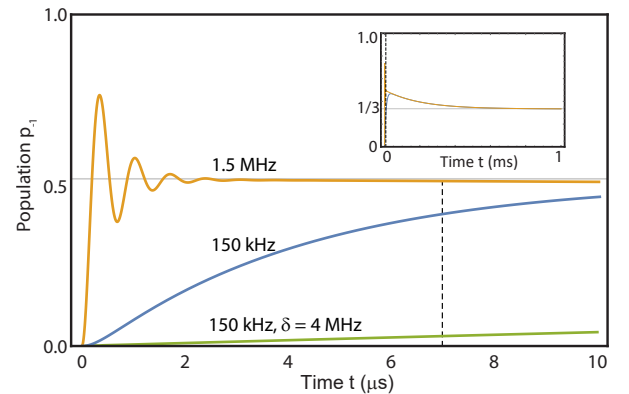

FIG. S10. Time-resolved dynamics under stress driving for  $\Omega_m/2\pi = 150$  kHz,  $\delta_{s,i}/2\pi = 0$  (blue) and  $1.5$  MHz,  $\delta_{s,i}/2\pi = 0$  (orange), and  $\Omega_m/2\pi = 150$  kHz,  $\delta_{s,i}/2\pi = 4$  MHz (green) with  $T_1 = 600 \mu\text{s}$ ,  $T_2^* = 0.5 \mu\text{s}$ . In all plots  $\delta_{m,s} = 0$ . The inset shows dynamics at longer times where populations reach steady-state due to  $T_1$  relaxation.

## V. SPIN-OPTOMECHANICS MEASUREMENTS

### A. Varying spin-mechanics detuning

To model the data in Fig. 4 in the main text, we use the model described above with several additional parameters to take into account our experimental conditions, which will be explained below. We begin with the simplest model, where the measured signal comes from a single NV that is initially perfectly polarized in  $|+1\rangle$ . In the measurement shown in Fig. 4 we scan the detuning  $\delta_{s,i}$  between the injection locked mechanical oscillations and the spin transition over the range  $2\pi \times [-2, 2]$  MHz. Each point corresponds to a  $7\mu\text{s}$ -long mechanical drive and a subsequent readout of  $p_{-1}$ . Figure S11 shows the simulated signal for three values of  $\Omega_m/2\pi = \{50, 1500, 600\}$  kHz in the ideal ‘on-resonance’ case where the intrinsic mechanical frequency prior to injection locking is resonant with the NV centers,  $\delta_{m,s} = 0$ . When we tune  $\delta_{s,i}$  the detuning between the lock frequency and the resonator’s intrinsic mechanical frequency,  $\delta_{m,i}$ , changes as well. This off-resonant driving causes a reduction in mechanical amplitude (see Fig. 2) and is taken into account in our model. We approximated the corresponding change via a function:

$$\Omega_m(\delta_{m,i}) = \frac{\Omega_m^0}{\sqrt{1 + 4\delta_{m,i}^2/\Gamma_{\text{tune}}^2}}, \quad (23)$$

where  $\Gamma_{\text{tune}}/2\pi = 380$  kHz is the FWHM of the mechanical resonator’s response to the injection locking observed in the experiment (see Fig. 2 in the main text). In Fig. S11, solid lines correspond to  $\Gamma_{\text{tune}}/2\pi = 380$  kHz while dashed lines have  $\Gamma_{\text{tune}}/2\pi = \infty$ . This figure shows that the finite bandwidth of the injection locking strongly affects the width of the data in Fig. 4, which at small  $\Omega_m$

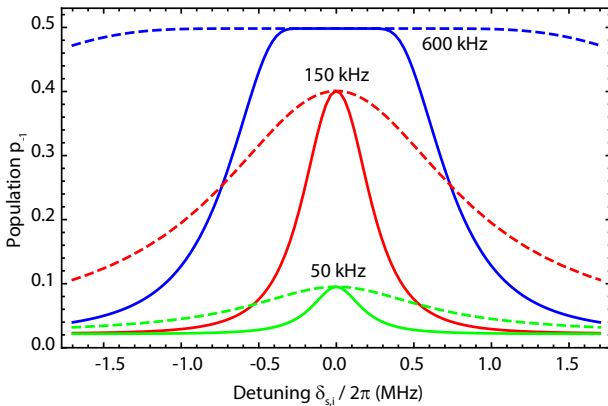

FIG. S11. Simulations similar to those used to generate theoretical curves in Fig. 4 of the main text. Mechanical driving time is  $7\mu\text{s}$ ,  $T_2^* = 0.5\mu\text{s}$ . Blue, red, and green curves corresponds to  $\Omega_m/2\pi = 50, 150, 600$  kHz, respectively. Solid lines show the injection locked PSD with  $\Gamma_{\text{tune}}/2\pi = 380$  kHz while dashed lines assume infinite bandwidth.

is close to  $\Gamma_{\text{tune}}$ , and broadens as  $\Omega_m$  increases.

Since the data was acquired over many days, slow drift in  $\omega_m$  was taken into consideration when fitting the experimental data. This drift manifests in the slightly larger FWHM of the stress-detuning dependence in the top panel of Figs. 4a and 4b compared to Fig. 2e (main text). Note that the inhomogeneous broadening of the ODMR spectra is taken into account in this model via  $T_2^*$ .

Figure 4 in the main text presents measurements done at the detuning  $\delta_{s,m} = 182$  kHz (Fig. 4a) and detuning  $\delta_{s,m} = -769$  kHz (Fig. 4b). Figure S12 shows additional data for the intermediate detuning  $\delta_{s,m} = -359$  kHz. The solid lines in Fig. S12 are theoretical predictions based on parameters ( $\Omega_m$  and  $r$ ) taken from fitting data in Fig. 4. Good agreement between the data and the model substantiates and supports the demonstration of optomechanical driving of spins.

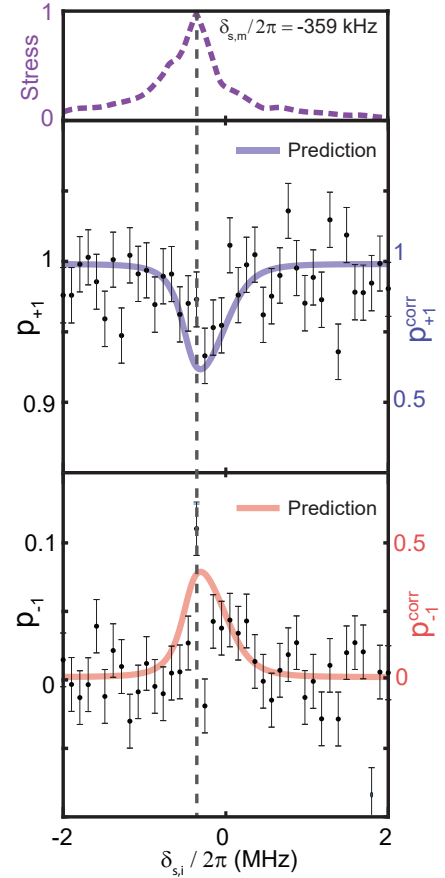

FIG. S12. Additional spin-optomechanics data, taken under the same conditions as the data in Fig. 4a in the main text, but with  $\delta_{s,m}/2\pi = -359$  kHz, i.e. further from resonance. Solid lines are theoretical predictions based on parameters extracted from fits to the data in Fig. 4a in the main text. The vertical dashed line shows the frequency where the injection locking tone is resonant with the mechanical resonator frequency.

## B. Fluorescence from the pedestal

Nitrogen vacancies in the pedestal enjoy better collection efficiency of their fluorescence due to geometrical effects: the pedestal funnels photons towards the objective. This causes an uneven profile of the photo-luminescence across the microdisk (Fig. 3c) with a bright spot in the center which affects the signal that we measure. Moreover, NVs in the pedestal experience vanishingly small stress (Fig. 2a) and do not change their spin projections during the  $7\mu\text{s}$ -long mechanical drive. To account for this effect we introduce a correction factor  $r$  equal to the fraction of photons collected from the pedestal relative to the total number of photons measured ( $r = 0$  means that no photons from the pedestal are detected). When fitting the data in Fig. 4 in the main text, we replace  $p_{-1}$  and  $p_{+1}$  obtained from solving the quantum master equation (Eq. 17) by  $(1-r)p_{-1}$  and  $r + (1-r)p_{+1}$ , respectively. This scaling takes into account the fact that we prepare and optomechanically drive  $|+1\rangle$ , and scales the signal contrast for both  $p_{-1}$  and  $p_{+1}$  equally. We refer to the rescaled populations as  $p_{\pm 1}^{\text{corr}}$ .

### *Effect on spatial dependence of signal*

In principle, measurements of population change as a function of the radial position could provide additional confidence on the value of  $r$ . There are two reasons why we have not been able to perform these measurements:

First, because  $r$  is in general a function of position it is non-trivial to extract changes in contrast stemming from the position dependent mechanical coupling. This is perhaps best illustrated by the fact that measured PL counts are actually enhanced at the edge of our microdisks owing to the devices' local optical density of states, as shown in Fig. 3c in the main text. Efforts to simulate the effect of the microdisk and its pedestal on NV PL are complicated by the need to both predict the effect of the device geometry on the green laser excitation spot, as well as the field radiated by the distribution of excited NVs. This is particularly challenging given that the exact geometry of the microdisk pedestal is not precisely known. A simpler and better approach in future work is to measure single NVs created within the microdisk using ion implantation or other methods. This will solve the 'pedestal problem' and allow working closer to the MD center where the stress is maximum.

A second challenge in our current experiment is achieving good SNR for reduced spin-mechanics coupling away from the centre of the microdisk. Stronger spin-phonon coupling in future work via improved device design or choice of spin qubit is required to solve this problem. These improvements are discussed in Sec. VI and in the main text.

## C. $|\pm 1\rangle$ nuclear transitions

Figure 4 focuses on only the  $|+1, 0_I\rangle \rightarrow |-1, 0_I\rangle$  transition. Although a total of three different nuclear-spin preserving transitions can be driven by phonons [11], it is not practical to observe all of them simultaneously in our setup. As described above, we manually tune the frequency of the  $|+1, 0_I\rangle \rightarrow |-1, 0_I\rangle$  transition to be resonant with the unlocked mechanical frequency by manually moving a permanent magnet and measuring ODMR after each adjustment to determine  $\omega_s$ . Typically several adjustments are required due to backlash in the micrometer used for position control. After adjusting the magnet, we use injection locking to change the mechanical frequency during the experiment (Fig. 2d). This is accompanied by a reduction of the mechanical amplitude and corresponding strain due to the finite bandwidth  $\Gamma_{\text{tune}}$  of the mechanical resonance (Fig. 2e). Since other nuclear transitions will be detuned by  $\delta f \approx 4\text{ MHz}$ , the corresponding mechanical Rabi frequency will be  $< \Omega_{\text{res}}/\sqrt{1 + 4 \cdot (\delta f/\Gamma_{\text{tune}})^2} \sim 10\text{ kHz}$ , where  $\Omega_{\text{res}} \approx 200\text{ kHz}$  is the estimated mechanical Rabi frequency when injection locking on-resonance.

This corresponds to a less than 5% change in the population. Taking into account the fluorescence factor  $r \sim 0.8$  this translates to a less than 1% change in the observed signal, well below the shot noise in Fig. 4, making it practically hard to observe these transitions without changing the position of the magnet.

We choose the  $|+1, 0_I\rangle \rightarrow |-1, 0_I\rangle$  transition over the other two mainly because we can engineer a 'magic'  $\pi$ -pulse for it (see Supplementary Section III). This is thanks to its equal detuning magnitude from the  $|+1, -1_I\rangle \rightarrow |-1, -1_I\rangle$  and  $|+1, +1_I\rangle \rightarrow |-1, +1_I\rangle$  transitions.

## D. Spin initialization and readout

The 'magic'  $\pi$ -pulse combined with the pulse sequence used in the experiment also allows us to omit the other two hyperfine sublevels in our analysis, as described below and shown in Figs. S13a and S13b for  $|+1\rangle$  and  $|-1\rangle$  readout, respectively:

**Initialization:** We initialize all NV spins into the  $|0\rangle$  electronic level via a  $5\mu\text{s}$ -long green pulse; populations of the nuclear sublevels remain almost equal during this step.

**State preparation:** (1) A 'magic'  $\pi$ -pulse transfers only  $|0, 0_I\rangle$  to  $|1, 0_I\rangle$ , leaving the other two nuclear sublevels virtually unaffected (see Fig. S13). (2) The stress field drives the transition  $|1, 0_I\rangle \rightarrow |-1, 0_I\rangle$ .

**Readout of  $|+1\rangle$ :** (a3) Another 'magic'  $\pi$ -pulse selectively drives  $|1, 0_I\rangle$  back to  $|0, 0_I\rangle$ . Without stress fields, all NV population is in the states  $|0, 0_I\rangle$ ,  $|0, -1_I\rangle$ , and  $|0, 1_I\rangle$  after this pulse. The resulting PL signal under green illumination corresponds to  $p_{+1} = 1$  in Fig. 4a. In the presence of the stress field, some NVs will populate

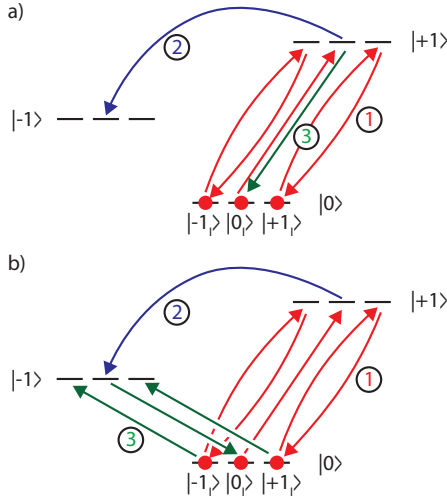

FIG. S13. Pulse sequences used during measurements of optomechanical driving of NV spins, showing their effect on populations of each hyperfine sublevel. Subfigures (a) and (b) show pulse sequences for reading the populations of the  $|+1\rangle$  and  $|-1\rangle$  states, respectively. Encircled numerical labels are referred to in the text describing each step of the process, with steps 1–3 corresponding to MW initialization, mechanical driving, and MW readout, respectively.

$|-1, 0_I\rangle$ . Since NVs in  $m_s = 1$  have dimmer PL, this corresponds to a dip in Fig. 4a.

**Readout of  $|-1\rangle$ :** (b3) A strong  $\pi$ -pulse on the  $|-1\rangle \rightarrow |0\rangle$  transition drives all three nuclear sublevels equally. Without stress fields, all NV population is the states  $|-1, 0_I\rangle$ ,  $|-1, -1_I\rangle$ , and  $|-1, +1_I\rangle$ . The PL signal under green illumination corresponds to  $p_{-1} = 0$  in Fig. 4a. In the presence of the stress field, some NVs will populate the level  $|0, 0_I\rangle$ . Since NVs in  $m_s = 0$  have brighter PL; this corresponds to a peak in Fig. 4a.

In both readout cases the PL signal is scaled using to the calibration provided by MW Rabi oscillations (Supplementary Section III) to represent the change in the populations of  $p_{-1} = |-1, 0_I\rangle$  and  $p_{+1} = |+1, 0_I\rangle$ . In this analysis we have neglected  $T_1$  processes of the  $|\pm 1_I\rangle$  hyperfine levels as it is expected that their population will change by less than 2% over a 7  $\mu$ s-long timescale due to  $T_1$  decay.

### E. Varying mechanical drive strength

Slow drift in  $\omega_m$ , when tracked, can provide an opportunity to measure the spin-mechanics interaction as a function of the mechanical oscillation amplitude, as in Fig. 4c in the main text. Data acquisition for this figure was made in runs spaced over a few months. During this time, a series of ‘spectral’ measurements of  $p_{\pm 1}$  as a function of  $\delta_{s,i}$  were made. Before each run, we measured the ODMR spectrum to precisely determine the NV spin transition frequency,  $\omega_s$ . If necessary we adjusted the

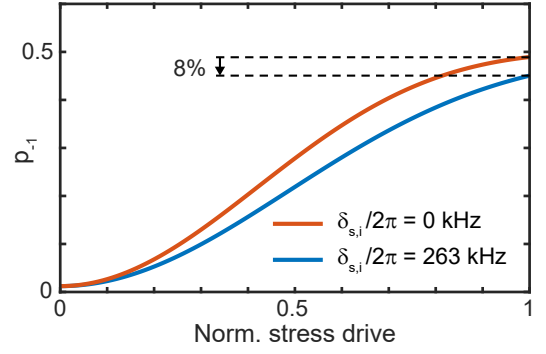

FIG. S14. Simulation of the  $|-1\rangle$  population for varying optomechanically driven stress field strength, after 7  $\mu$ s of mechanical driving. Spin-mechanics detuning values,  $\delta_{s,i}$ , corresponding to the on-resonance condition (red line) and the condition used for the data in Fig. 4c in the main text (blue line) are shown.

magnet position and repeated the ODMR measurement until reaching an acceptable  $|\delta_{s,m}|$ . We then performed the spectral measurement over a period of around 14 hours, during which time  $\omega_s$  typically did not vary appreciably. During each spectral measurement, the slowly drifting  $\omega_m$  was monitored continuously. Due to the resulting variation in  $\delta_{s,m}$ , for a chosen detuning  $\delta_{s,i}$  between the injection locked mechanical frequency and the spin transition, the strength of the stress field and  $\Omega_m$  varied, as it depends on  $\delta_{m,i} = \delta_{s,i} - \delta_{s,m}$  (Fig. 2e in the main text and Eq. (23)). By accumulating several runs of  $p_{\pm 1}$  spectra, and using post-processing to select data points from each spectra at constant  $\delta_{s,i}$  and varying  $\delta_{m,i}$ , we generated Fig. 4c in the main text. Note that in each spectral measurement the amplitude of self-oscillation when  $\delta_{m,i} = 0$  was monitored and stabilized.

Over the course of our experiment, we accumulated the largest amount of data for varying  $\delta_{m,i}$  and fixed  $\delta_{s,i}$  at non-zero detuning  $\delta_{s,i}/2\pi = 263$  kHz. It is at this value of  $\delta_{s,i}$  where our data set provides the optimal combination of dynamic range of  $\Omega_m$  and signal to noise when generating the plots in Fig. 4c in the main text. In Fig. S14 we show that this choice of non-zero  $\delta_{s,i}$  is expected to only reduce the maximum change in the measured signal by 8% when compared with the  $\delta_{s,i} = 0$  case.

## VI. TOWARDS A DETERMINISTIC SPIN-OPTOMECHANICAL INTERFACE

A reversible interface between telecom photons and quantum memories is a key building block for creating quantum networks [13]. Our work shows the potential of spin-optomechanical devices for this purpose. However, the system we use in this proof-of-principle demonstration—ground state spins of NV centers coupled to a diamond microdisk—does not yet operate in the quantum regime needed for reversible operation. Below

we detail improvements that in future will allow operation in this regime.

### A. Requirements for coherent spin-optomechanics

An interface between two quantum systems can be characterized by cooperativity  $C = 4g^2/\gamma_1\gamma_2$ , where  $g$  is the coupling rate between the systems and  $\gamma_{1,2}$  are the linewidths of each system. When  $C > 1$ , the systems can coherently interact, despite their internal decoherence. Our spin-optomechanical device couples three quantum systems. Its two interfaces are characterized by spin-phonon cooperativity  $C_{sm}$  and phonon-photon cooperativity  $C_{om}$ . It can be shown that in such a two-interface system, the transduction efficiency ( $\eta$ ) from a photon to a spin is [13]:

$$\eta = \frac{4C_{sm}C_{om}}{(1 + C_{sm} + C_{om})^2}. \quad (24)$$

For  $C_{sm}, C_{om} \gg 1$ , near unity transduction efficiency is possible. Equation (24) assumes that both couplings are always on, which results in the requirement that  $C_{sm} = C_{om}$  for optimal efficiency. Other proposals [17, 18] lift

this restriction by employing temporal control of coupling rates.

Our current system satisfies  $C_{om} > 1$ . However, it has  $C_{sm} \ll 1$ . By using different spin-qubits and modifying our cavity optomechanical device geometry, as illustrated in Fig. S15, we can boost both of these cooperativities and realize a coherent spin-photon interface with  $\eta \approx 1$ .

### Cryogenic operation

The discussion in this section assumes that the device is operated in a cryogenic environment that eliminates thermal phonons populating the mechanical resonator. For GHz frequency mechanical resonators, this has been achieved in commercially available dilution refrigerators with base temperatures ranging from 10 - 100 mK [16, 19, 20]. In this regime,  $\gamma_m$  is the relevant mechanical decoherence rate when calculating  $C_{om}$  and  $C_{sm}$ . It is also possible to operate at higher base temperatures, for example in 4K liquid-He cryostats, and employ optomechanical cooling to eliminate thermal phonons [21]. However, this cooling via damping is accompanied by increased  $\gamma_m$ . Finally, we note that in the presence of thermal phonon population  $n_{th}$ ,  $\gamma_m \rightarrow \gamma_m(1 + n_{th})$  when calculating  $C_{sm}$  and  $C_{om}$ . This penalty can in principle be overcome by reducing decoherence rates and increasing coupling rates of the system.

### B. Spin-phonon interactions ( $C_{sm}$ )

Given the parameters describing the spin-phonon dynamics of our system (mechanical decay rate  $\gamma_m/2\pi = f_m/Q_m \approx 0.5$  MHz, spin dephasing rate  $\gamma_{spin}/2\pi \approx 1$  MHz, coupling rate between a single NV ground state spin and a single phonon  $g_{sm}/2\pi \approx 10$  Hz) we find that it possesses  $C_{sm} = 4g_{sm}^2/\gamma_m\gamma_{spin} \approx 10^{-9}$ , far smaller than required to realize a coherent quantum interface. As  $g_{sm} \propto g_{stress}/\sqrt{V_m}$ , where  $g_{stress}$  is the spin qubit's sensitivity to stress and  $V_m$  is the device's mechanical mode volume,  $g_{sm}$  can be increased both by using spins with enhanced intrinsic strain coupling, and by reducing the mechanical resonator dimensions. Mechanical damping  $\gamma_m$  is a function of mechanical resonator design, and can be improved by adopting geometries that restrict the leakage of phonons out of the resonator. Diamond spin qubit decoherence rates are typically in the range of  $1/\gamma_{spin} = 1 - 10 \mu s$  for qubits in practical devices. Although they can be increased in some cases through improvements in material quality, maintaining such high coherence can be challenging in photonic devices. In this discussion we focus on increasing  $C_{sm}$  through improvements to  $g_{sm}$  and  $\gamma_m$ . In doing so it is immediately viable to increase  $C_{sm}$  from  $\approx 10^{-9}$  to  $> 100$  using already demonstrated spin qubits and devices. This discussion also assumes that the system has a single spin or a distinguishable spin ensemble. In the case of an indistin-

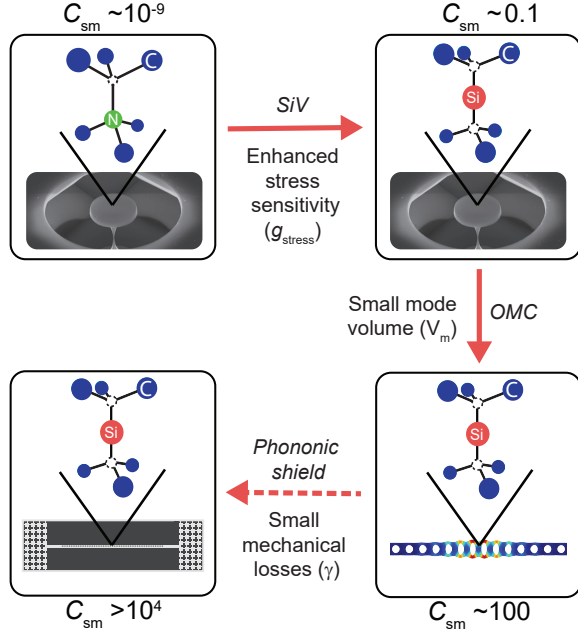

FIG. S15. The proposed path for increasing the spin-mechanical cooperativity  $C_{sm}$ . First, replacing NV centers with SiV centers will result in a higher sensitivity to stress bringing  $C_{sm} \approx 0.2$ . Next, using optomechanical crystals (OMC) rather than microdisks reduces mechanical mode volume, leading to  $C_{sm} \approx 100$ . Since diamond OMC [14] and mechanical control of SiV centers [15] have been already realized, the target of  $C_{sm} = 100$  is feasible. Adding phonon shielding to diamond OMC should result in significantly smaller mechanical losses (as has been shown in Si devices [16]) with the projected  $C_{sm} > 10^4$ .



3.6 MHz when coupled to SiV spin qubits through direct coupling [36]. Similarly, Neuman et al. [17] predict  $g_{\text{sm}}/2\pi \approx 2.4$  MHz for a diamond optomechanical crystal coupled to an SiV spin via the microwave Raman approach described above. Diamond optomechanical crystal cavities have similar or better  $\gamma_{\text{m}}$  as microdisks [14], with  $\gamma_{\text{m}}/2\pi \approx 0.5$  MHz observed at dilution fridge temperatures [37]. For these parameters we expect  $C_{\text{sm}} \approx 60 - 120$  for an SiV coupled to an optomechanical crystal cavity.

Phonon assisted optical Raman coupling of an NV to an optomechanical crystal would have a similar cooperativity. However, NVs with sharp optical transitions have not yet been reliably observed in nanoscale cavities.

#### *Phononic shields: reducing $\gamma_{\text{m}}$*

Mechanical resonators can be designed to possess ultralow  $\gamma_{\text{m}}$  through phononic bandgap engineering. Phononic bandgaps restrict the leakage of phonons, which unlike photons, do not scatter out of devices into the surrounding vacuum. Optomechanical crystal cavities can be embedded within phononic crystal shields to reduce  $\gamma_{\text{m}}$ . This approach has led to demonstration of  $\gamma_{\text{m}}$  below 1 kHz in silicon optomechanical crystal cavities [16]. If similar phononic crystals can be created in diamond to reduce  $\gamma_{\text{m}}$  to this level, a further increase in  $C_{\text{sm}}$  by approximately  $\times 1000$  may be possible.

### C. Phonon-photon interactions ( $C_{\text{om}}$ )

Realizing coherent photon-phonon intraconversion requires  $C_{\text{om}} > 1$  for a device cooled near its mechanical quantum ground state ( $n_{\text{th}} \approx 0$ ), where

$$C_{\text{om}} = N_{\text{cav}} \frac{4g_{\text{om}}^2}{\kappa\gamma_{\text{m}}}. \quad (25)$$

Here  $\kappa$  is the energy decay rate of the optical resonance and  $N_{\text{cav}}$  is the number of photons coupled into the optical cavity mode by a classical pump laser. When the pump laser is red-detuned by the mechanical frequency from the optical mode, a single telecom photon resonant with the cavity can efficiently scatter into the pump mode while simultaneously generating a phonon. This operating condition is often referred to as the optomechanically induced transparency (OMIT) configuration, and has been demonstrated in diamond microdisks with  $C_{\text{om}} > 3$  [29] as well as diamond optomechanical crystal cavities with  $C_{\text{om}} > 10$  [14]. These demonstrations were achieved in devices operating in ambient conditions and thus have  $n_{\text{th}} \gg 1$ . Cooling the devices to dilution fridge temperatures, as demonstrated in Ref. [37] with diamond optomechanical crystals, will reduce  $n_{\text{th}} \ll 1$ . An outstanding challenge is demonstrating (OMIT) in these devices without increasing  $n_{\text{th}} > C_{\text{om}}$  via optical absorption. Silicon optomechanical devices satisfying this condition have been already been demonstrated at mK temperatures [20, 38].

Looking forward, adding a phononic shield to an OMC [16] to reduce the mechanical decay rate to  $\gamma_{\text{m}}/2\pi \approx 1$  kHz, as discussed above, can enable  $C_{\text{om}} \approx 1$  even without the pump laser ( $N_{\text{cav}} = 1$ ) at mK temperatures. Reducing  $\gamma_{\text{m}}$  would also allow the more general condition for coherent photon-phonon conversion,  $C_{\text{om}} > 1 + n_{\text{th}}$ , to be routinely satisfied at elevated temperatures.

### D. Summary

To summarize, as illustrated in Fig. S15, using well-understood diamond silicon-vacancy centers placed in already demonstrated diamond optomechanical devices, one can simultaneously achieve  $C_{\text{sm}} > 1$  and  $C_{\text{om}} > 1$  at mK temperatures. This quantum regime could also in principle be realized with NVs using parametric coupling to spins via optical excited state transitions.

- 
- [1] M. Mitchell, B. Khanaliloo, D. P. Lake, T. Masuda, J. P. Hadden, and P. E. Barclay, Single-crystal diamond low-dissipation cavity optomechanics, *Optica* **3**, 963 (2016).
  - [2] M. Mitchell, D. P. Lake, and P. E. Barclay, Optomechanically amplified wavelength conversion in diamond microcavities, *Optica* **6**, 832 (2019), arXiv:1902.07763.
  - [3] V. M. Acosta, E. Bauch, M. P. Ledbetter, C. Santori, K.-M. C. Fu, P. E. Barclay, R. G. Beausoleil, H. Linet, J. F. Roch, F. Treussart, S. Chemerisov, W. Gawlik, and D. Budker, Diamonds with a high density of nitrogen-vacancy centers for magnetometry applications, *Phys. Rev. B* **80**, 115202 (2009).
  - [4] D. P. Lake, M. Mitchell, Y. Kamaliddin, and P. E. Barclay, Optomechanically Induced Transparency and Cooling in Thermally Stable Diamond Microcavities, *ACS Photonics* **5**, 782 (2018).
  - [5] D. S. Weiss, V. Sandoghdar, J. Hare, V. Lefèvre-Seguin, J.-M. Raimond, and S. Haroche, Splitting of high-Q Mie modes induced by light backscattering in silica microspheres, *Optics Letters* **20**, 1835 (1995).
  - [6] K. Srinivasan, P. E. Barclay, O. Painter, J. Chen, A. Y. Cho, and C. Gmachl, Experimental demonstration of a high quality factor photonic crystal microcavity, *Applied Physics Letters* **83**, 1915 (2003).
  - [7] M. Aspelmeyer, T. J. Kippenberg, and F. Marquardt, Cavity optomechanics, *Reviews of Modern Physics* **86**, 1391 (2014).
  - [8] J.-P. Tetienne, L. Rondin, P. Spinicelli, M. Chipaux, T. Debuisschert, J.-F. Roch, and V. Jacques, Magnetic-field-dependent photodynamics of single NV defects in diamond: an application to qualitative all-optical magnetic imaging, *New Journal of Physics* **14**, 103033 (2012).

- [9] V. Jacques, P. Neumann, J. Beck, M. Markham, D. Twitchen, J. Meijer, F. Kaiser, G. Balasubramanian, F. Jelezko, and J. Wrachtrup, Dynamic polarization of single nuclear spins by optical pumping of nitrogen-vacancy color centers in diamond at room temperature., *Physical review letters* **102**, 057403 (2009).
- [10] R. Fischer, A. Jarmola, P. Kehayias, and D. Budker, Optical polarization of nuclear ensembles in diamond, *Physical Review B* **87**, 125207 (2013).
- [11] E. R. Macquarrie, T. A. Gosavi, N. R. Jungwirth, S. A. Bhawe, and G. D. Fuchs, Mechanical spin control of nitrogen-vacancy centers in diamond, *Physical Review Letters* **111**, 227602 (2013), arXiv:1306.6356.
- [12] P. Udvarhelyi, V. O. Shkolnikov, A. Gali, G. Burkard, and A. Pályi, Spin-strain interaction in nitrogen-vacancy centers in diamond, *Physical Review B* **98**, 75201 (2018).
- [13] N. Lauk, N. Sinclair, S. Barzanjeh, J. P. Covey, M. Saffman, M. Spiropulu, and C. Simon, Perspectives on quantum transduction, *Quantum Science and Technology* **5**, 20501 (2020).
- [14] M. J. Burek, J. D. Cohen, S. M. Meenehan, N. El-Sawah, C. Chia, T. Ruelle, S. Meesala, J. Rochman, H. A. Atikian, M. Markham, D. J. Twitchen, M. D. Lukin, O. Painter, and M. Lončar, Diamond optomechanical crystals, *Optica* **3**, 1404 (2016).
- [15] S. Maity, L. Shao, S. Bogdanović, S. Meesala, Y.-I. Sohn, N. Sinclair, B. Pingault, M. Chalupnik, C. Chia, L. Zheng, K. Lai, and M. Lončar, Coherent acoustic control of a single silicon vacancy spin in diamond, *Nature Communications* **11**, 193 (2020).
- [16] G. S. MacCabe, H. Ren, J. Luo, J. D. Cohen, H. Zhou, A. Sipahigil, M. Mirhosseini, and O. Painter, Nano-acoustic resonator with ultralong phonon lifetime, *Science* **370**, 840 (2020).
- [17] T. Neuman, M. Eichenfield, M. Trusheim, L. Hackett, P. Narang, and D. Englund, A Phononic Bus for Coherent Interfaces Between a Superconducting Quantum Processor, Spin Memory, and Photonic Quantum Networks (2020), arXiv:2003.08383 [quant-ph].
- [18] M. Mirhosseini, A. Sipahigil, M. Kalaei, and O. Painter, Superconducting qubit to optical photon transduction, *Nature* **588**, 599 (2020).
- [19] J. D. Cohen, S. M. Meenehan, G. S. MacCabe, S. Gröblacher, A. H. Safavi-Naeini, F. Marsili, M. D. Shaw, and O. Painter, Phonon counting and intensity interferometry of a nanomechanical resonator, *Nature* **520**, 522 (2015).
- [20] A. Wallucks, I. Marinković, B. Hensen, R. Stockill, and S. Gröblacher, A quantum memory at telecom wavelengths, *Nature Physics* **16**, 772 (2020).
- [21] J. Chan, T. P. M. Alegre, A. H. Safavi-Naeini, J. T. Hill, A. Krause, S. Gröblacher, M. Aspelmeyer, and O. Painter, Laser cooling of a nanomechanical oscillator into its quantum ground state, *Nature* **478**, 89 (2011).
- [22] H. Wang and I. Lekavicius, Coupling spins to nanomechanical resonators: Toward quantum spin-mechanics (2020), arXiv:2011.09990 [cond-mat.mes-hall].
- [23] Hepp, *Electronic Structure of the Silicon Vacancy Color Center in Diamond*, Ph.D. thesis (2014).
- [24] A. Sipahigil, R. E. Evans, D. D. Sukachev, M. J. Burek, J. Borregaard, M. K. Bhaskar, C. T. Nguyen, J. L. Pacheco, H. A. Atikian, C. Meuwly, R. M. Camacho, F. Jelezko, E. Bielejec, H. Park, M. Lončar, and M. D. Lukin, An integrated diamond nanophotonics platform for quantum optical networks, *Science* **354**, 847 (2016).
- [25] D. Sukachev, Photon-mediated interactions between quantum emitters in a diamond nanocavity, in *Proceedings of SPIE - The International Society for Optical Engineering*, Vol. 10904 (2019).
- [26] R. E. Evans, A. Sipahigil, D. D. Sukachev, A. S. Zibrov, and M. D. Lukin, Narrow-Linewidth Homogeneous Optical Emitters in Diamond Nanostructures via Silicon Ion Implantation, *Physical Review Applied* **5**, 044010 (2016), arXiv:1512.03820.
- [27] S. Meesala, Y.-I. Sohn, H. A. Atikian, M. J. Burek, S. Kim, J. Choy, and M. Loncar, Strain coupling of diamond nitrogen vacancy centers to nanomechanical resonators, in *CLEO:2015* (OSA, Washington, D.C., 2015) p. FTh3B.4.
- [28] M. A. Lemonde, S. Meesala, A. Sipahigil, M. J. A. Schuetz, M. D. Lukin, M. Loncar, and P. Rabl, Phonon networks with SiV centers in diamond waveguides, *Physical Review Letters* **120**, 213603 (2018).
- [29] D. P. Lake, M. Mitchell, D. D. Sukachev, and P. E. Barclay, Processing light with an optically tunable mechanical memory, *Nature Communications* **12**, 1 (2021).
- [30] J. N. Becker, B. Pingault, D. Groß, M. Gündoğan, N. Kukharchyk, M. Markham, A. Edmonds, M. Atatüre, P. Bushev, and C. Becher, All-Optical Control of the Silicon-Vacancy Spin in Diamond at Millikelvin Temperatures, *Physical Review Letters* **120**, 053603 (2018).
- [31] D. A. Golter, T. Oo, M. Amezcua, I. Lekavicius, K. A. Stewart, and H. Wang, Coupling a Surface Acoustic Wave to an Electron Spin in Diamond via a Dark State, *Physical Review X* **6**, 41060 (2016).
- [32] S. Chakravarthi, C. Pederson, Z. Kazi, A. Ivanov, and K.-M. C. Fu, Spectrally stable near-surface implanted nitrogen vacancy centers in diamond and the role of surface proximity (2021), arXiv:2105.09483 [cond-mat.mes-hall].
- [33] M. Eichenfield, J. Chan, R. M. Camacho, K. J. Vahala, and O. Painter, Optomechanical crystals, *Nature* **462**, 78 (2009).
- [34] J. V. Cady, O. Michel, K. W. Lee, R. N. Patel, C. J. Sarabalis, A. H. Safavi-Naeini, and A. C. B. Jayich, Diamond optomechanical crystals with embedded nitrogen-vacancy centers, *Quantum Science and Technology* **4**, 024009 (2019).
- [35] C. Chia, M. Chalupnik, and M. Loncar, Engineering spin-phonon coupling rates for the silicon vacancy center in diamond phononic crystal cavities, in *CLEO:QELS Fundamental Science* (Optical Society of America, 2021) p. JW4L.1.
- [36] S. Meesala, Y.-I. Sohn, H. A. Atikian, S. Kim, M. J. Burek, J. T. Choy, and M. Lončar, Enhanced Strain Coupling of Nitrogen-Vacancy Spins to Nanoscale Diamond Cantilevers, *Physical Review Applied* **5**, 34010 (2016).
- [37] G. Joe, C. Chia, M. Chalupnik, B. Pingault, S. Meesala, E. Cornell, D. Assumpcao, B. Machiels, and M. Loncar, Diamond phononic crystals with silicon-vacancy centers at cryogenic temperatures, in *CLEO:QELS Fundamental Science* (Optical Society of America, 2021) p. FTh4M.1.
- [38] M. Forsch, R. Stockill, A. Wallucks, I. Marinković, C. Gärtner, R. A. Norte, F. van Otten, A. Fiore, K. Srinivasan, and S. Gröblacher, Microwave-to-optics conversion using a mechanical oscillator in its quantum ground state, *Nature Physics* **16**, 69 (2020).
